# Supplementary material for: Compressed Vision for Efficient Video Understanding
Source: arXiv:2210.02995 source file (2022-10-06)

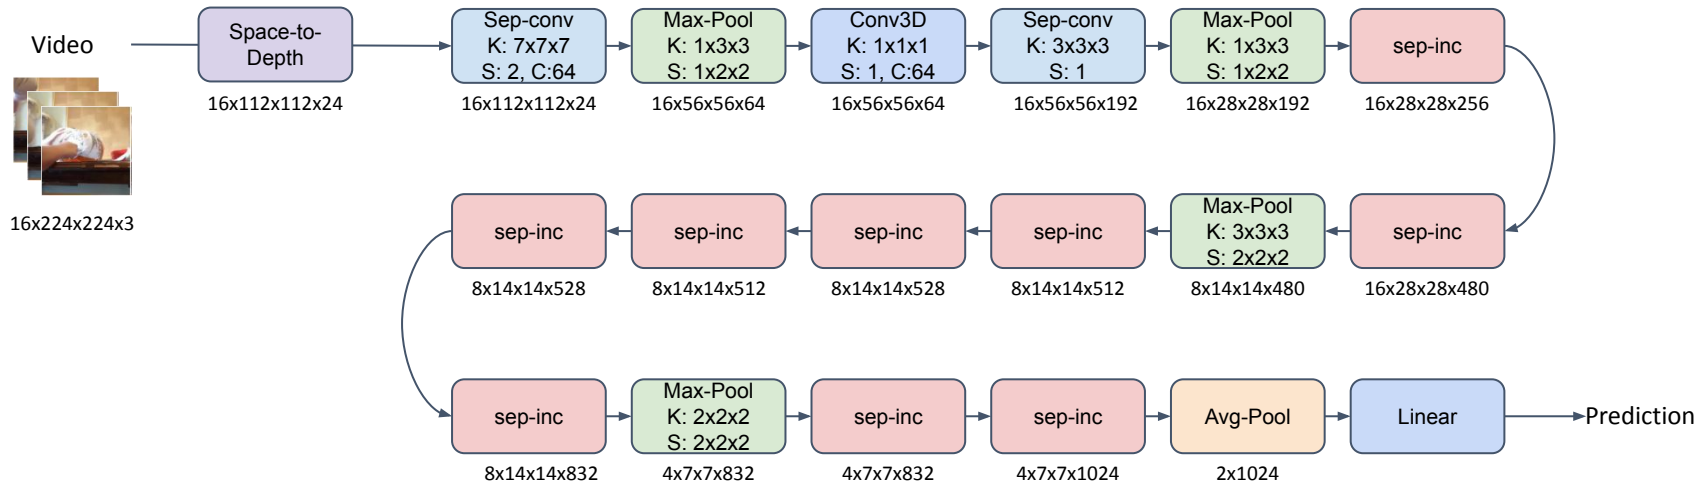

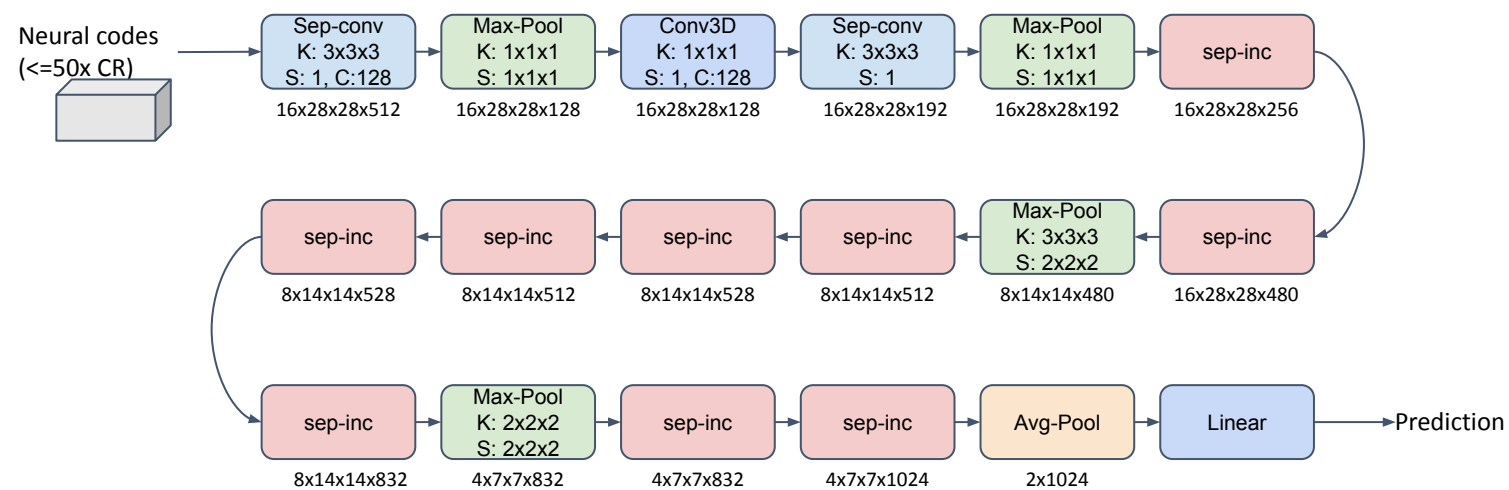

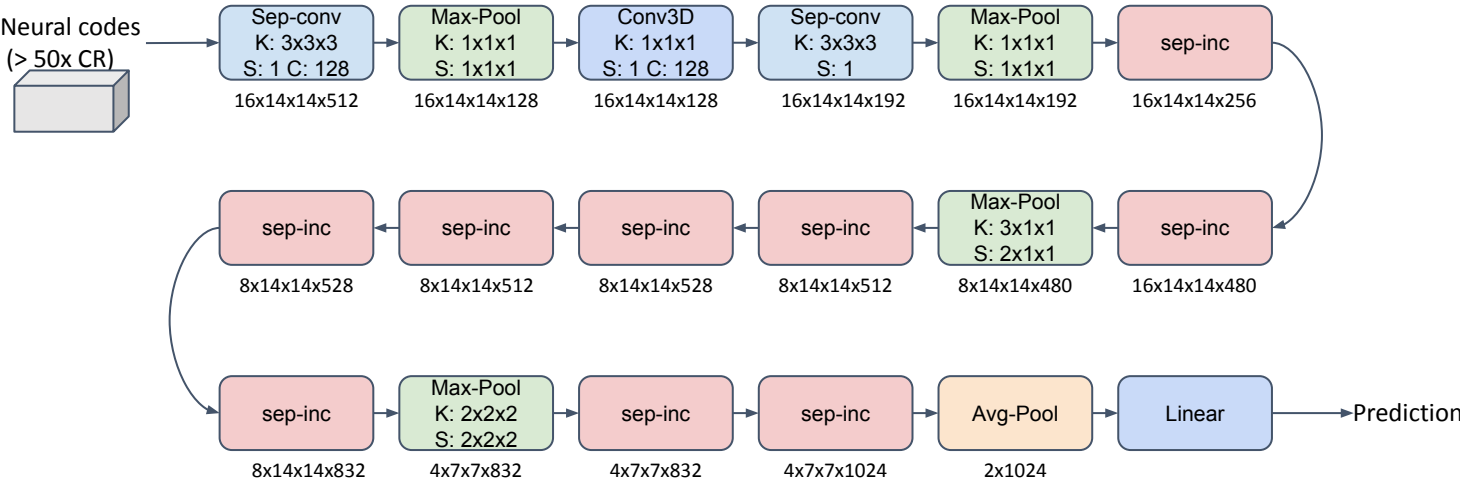

Supplement: Supplementary file 1 [file s3d_figures.pdf]
